# Supplementary material for: FILM: Framework for Imbalanced Learning Machines based on a new unbiased performance measure and a new ensemble-based technique
Source: arXiv:2503.04370 source file (2025-03-06)
Supplement: Supplementary file 1 [file SupplementaryIPIP.pdf]

# Supplementary material

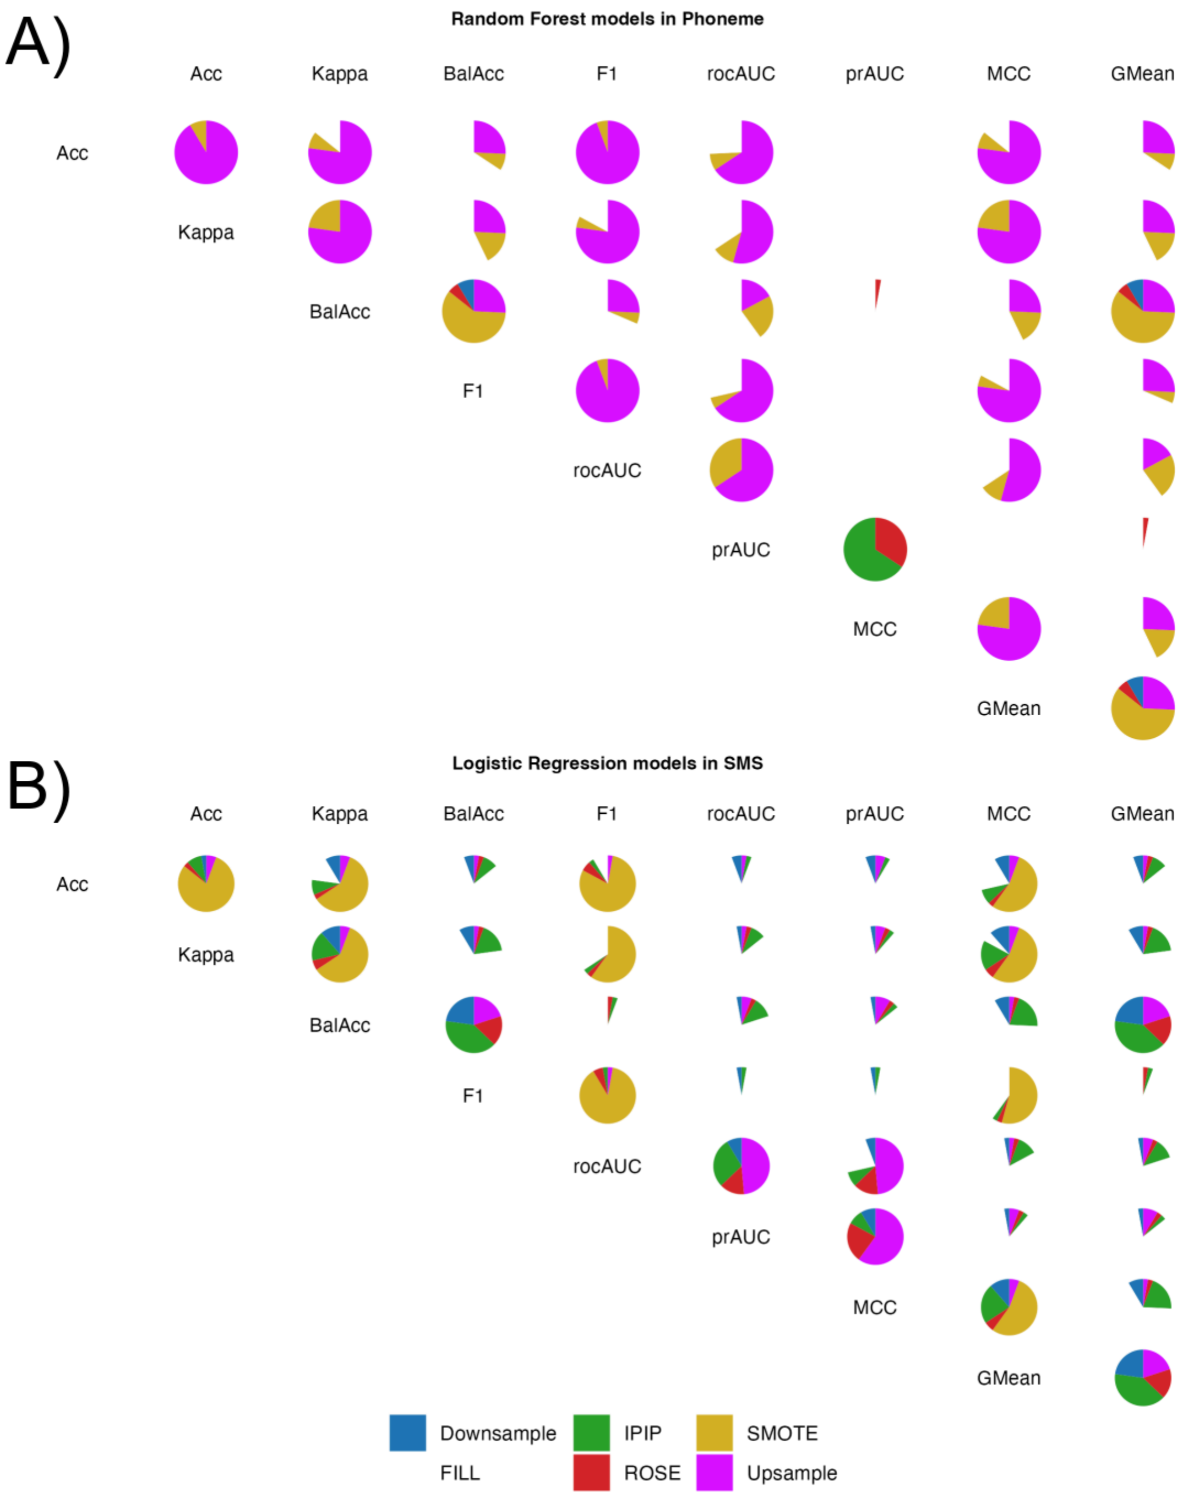


Supplementary Figure S1: A) Concordance plot of the Phoneme dataset using Random Forest. B) Concordance plot of the SMS dataset using Logistic Regression models.

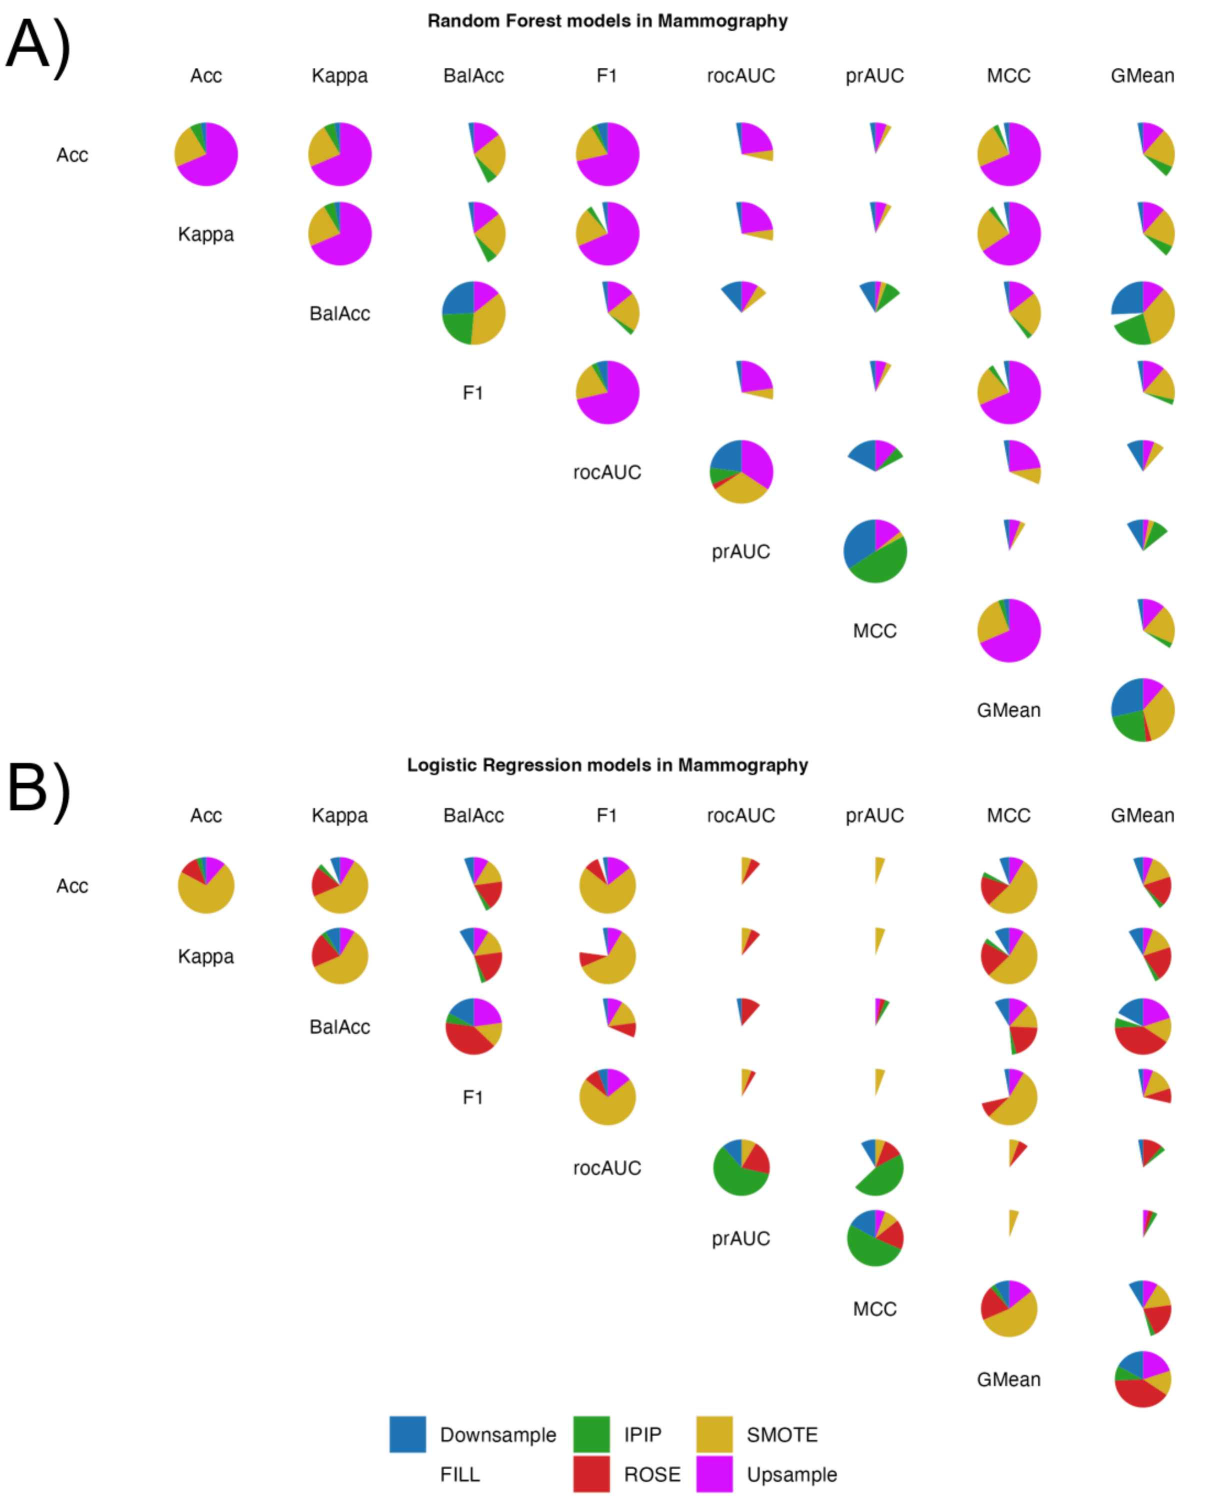


Supplementary Figure S2: A) Concordance plot of the Mammography dataset using Random Forest. B) Concordance plot of the Mammography dataset using Logistic Regression models.

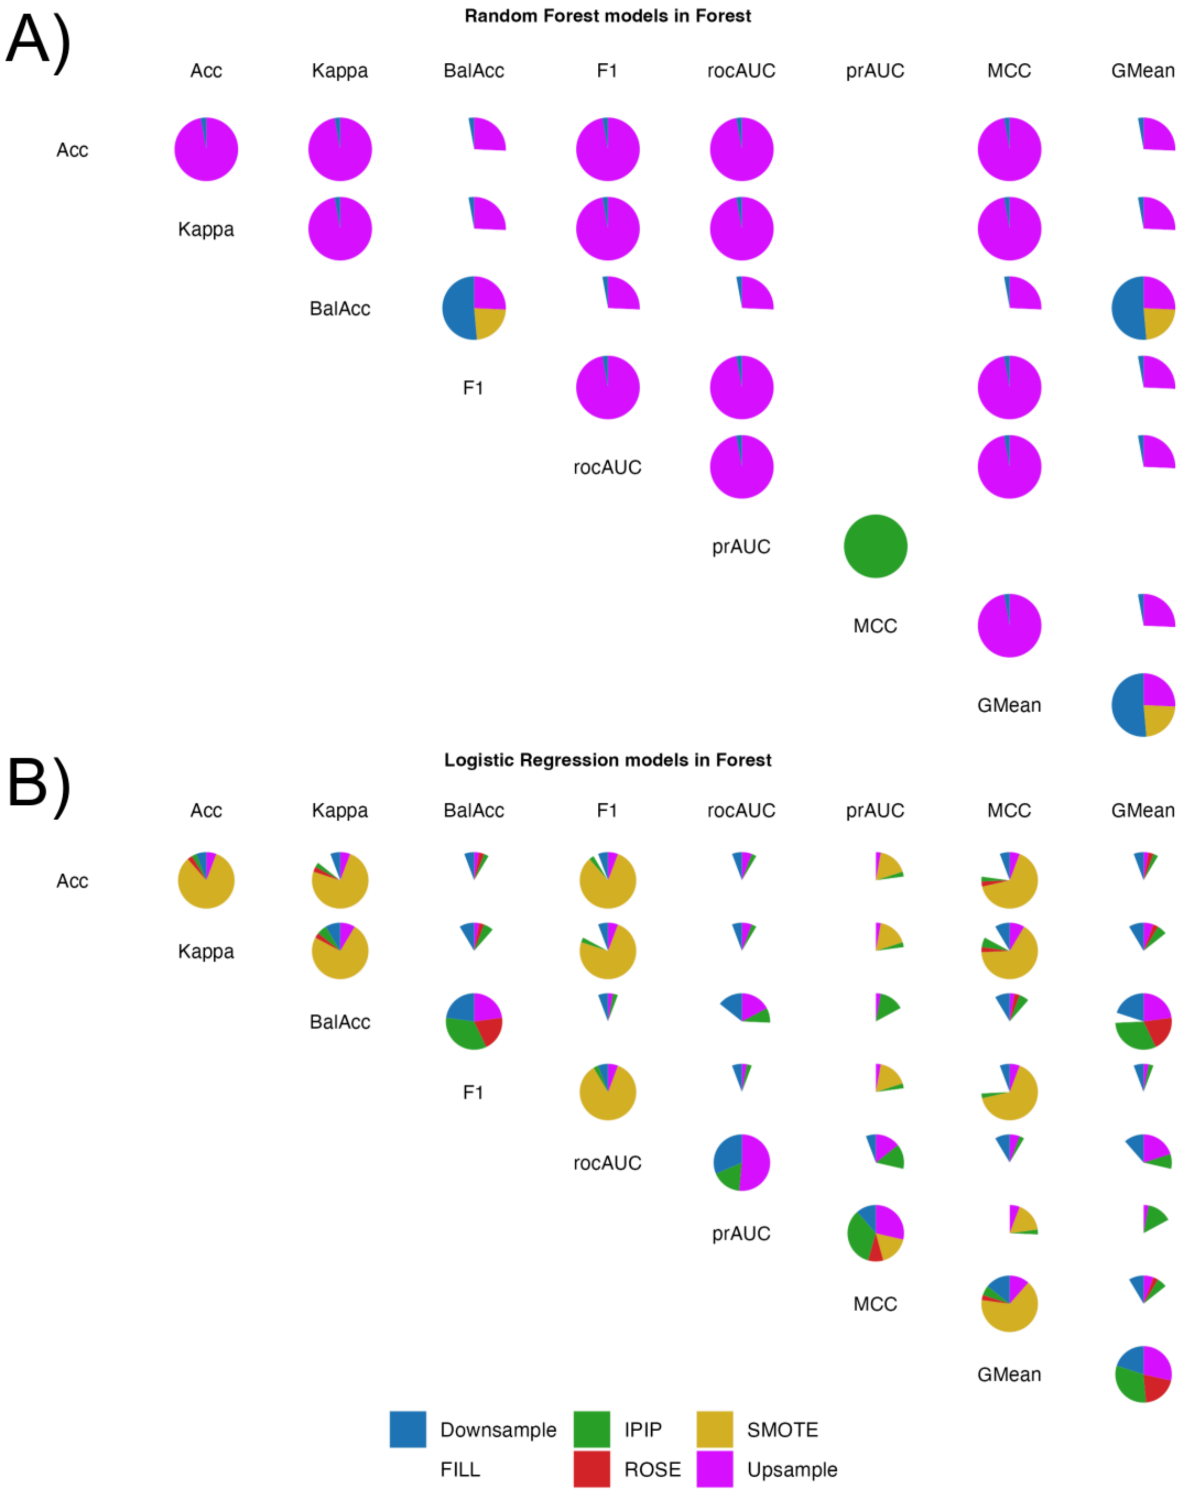


Supplementary Figure S3: A) Concordance plot of the Forest dataset using Random Forest. B) Concordance plot of the Forest dataset using Logistic Regression models.

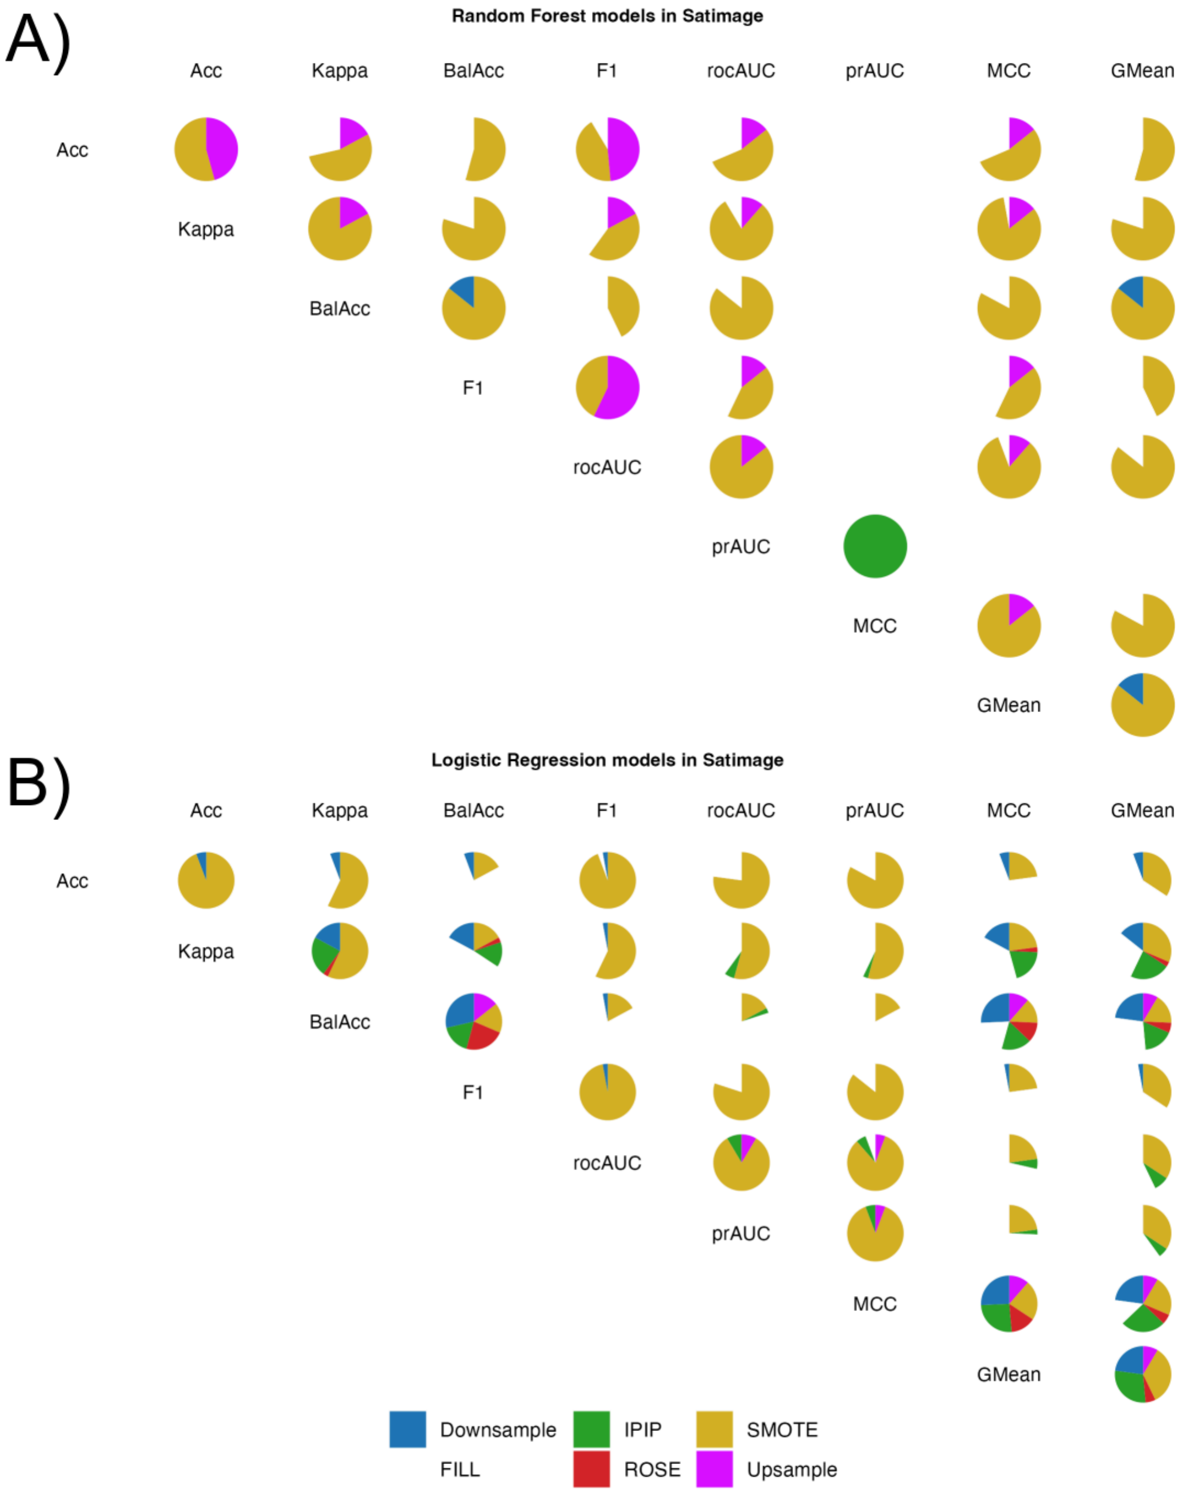


Supplementary Figure S4: A) Concordance plot of the Satimage dataset using Random Forest. B) Concordance plot of the Satimage dataset using Logistic Regression models.

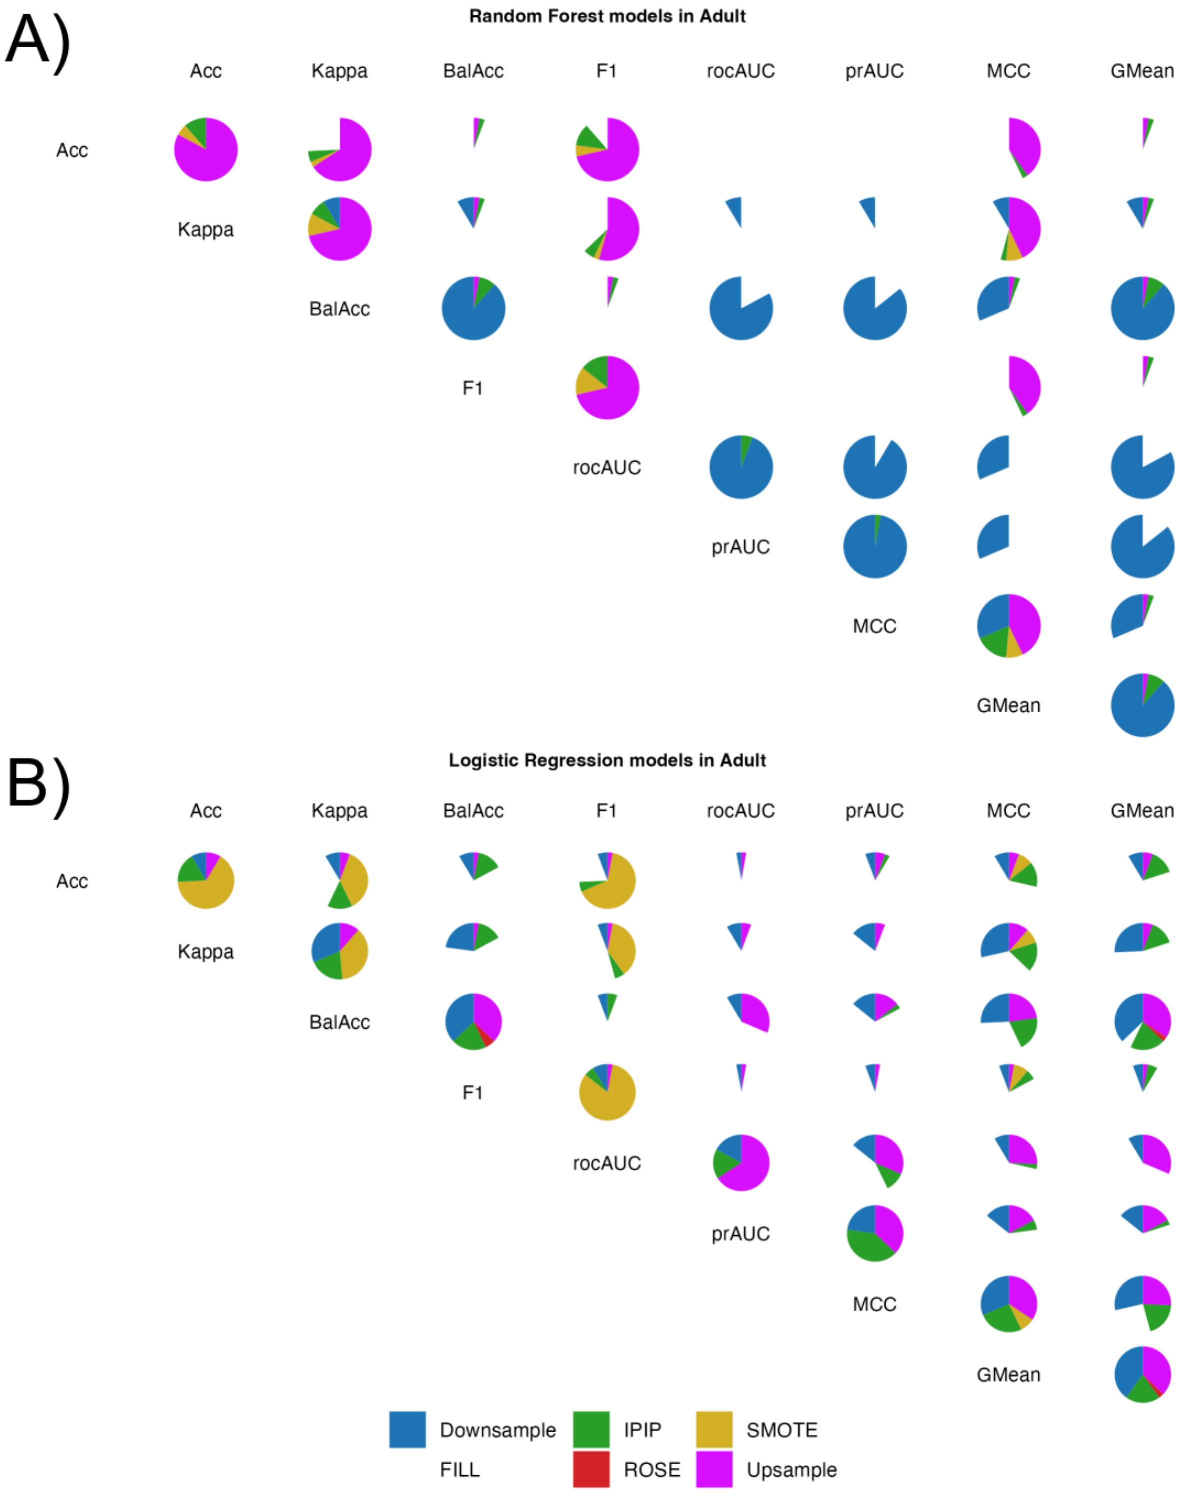


Supplementary Figure S5: A) Concordance plot of the Adult dataset using Random Forest. B) Concordance plot of the Adult dataset using Logistic Regression models.

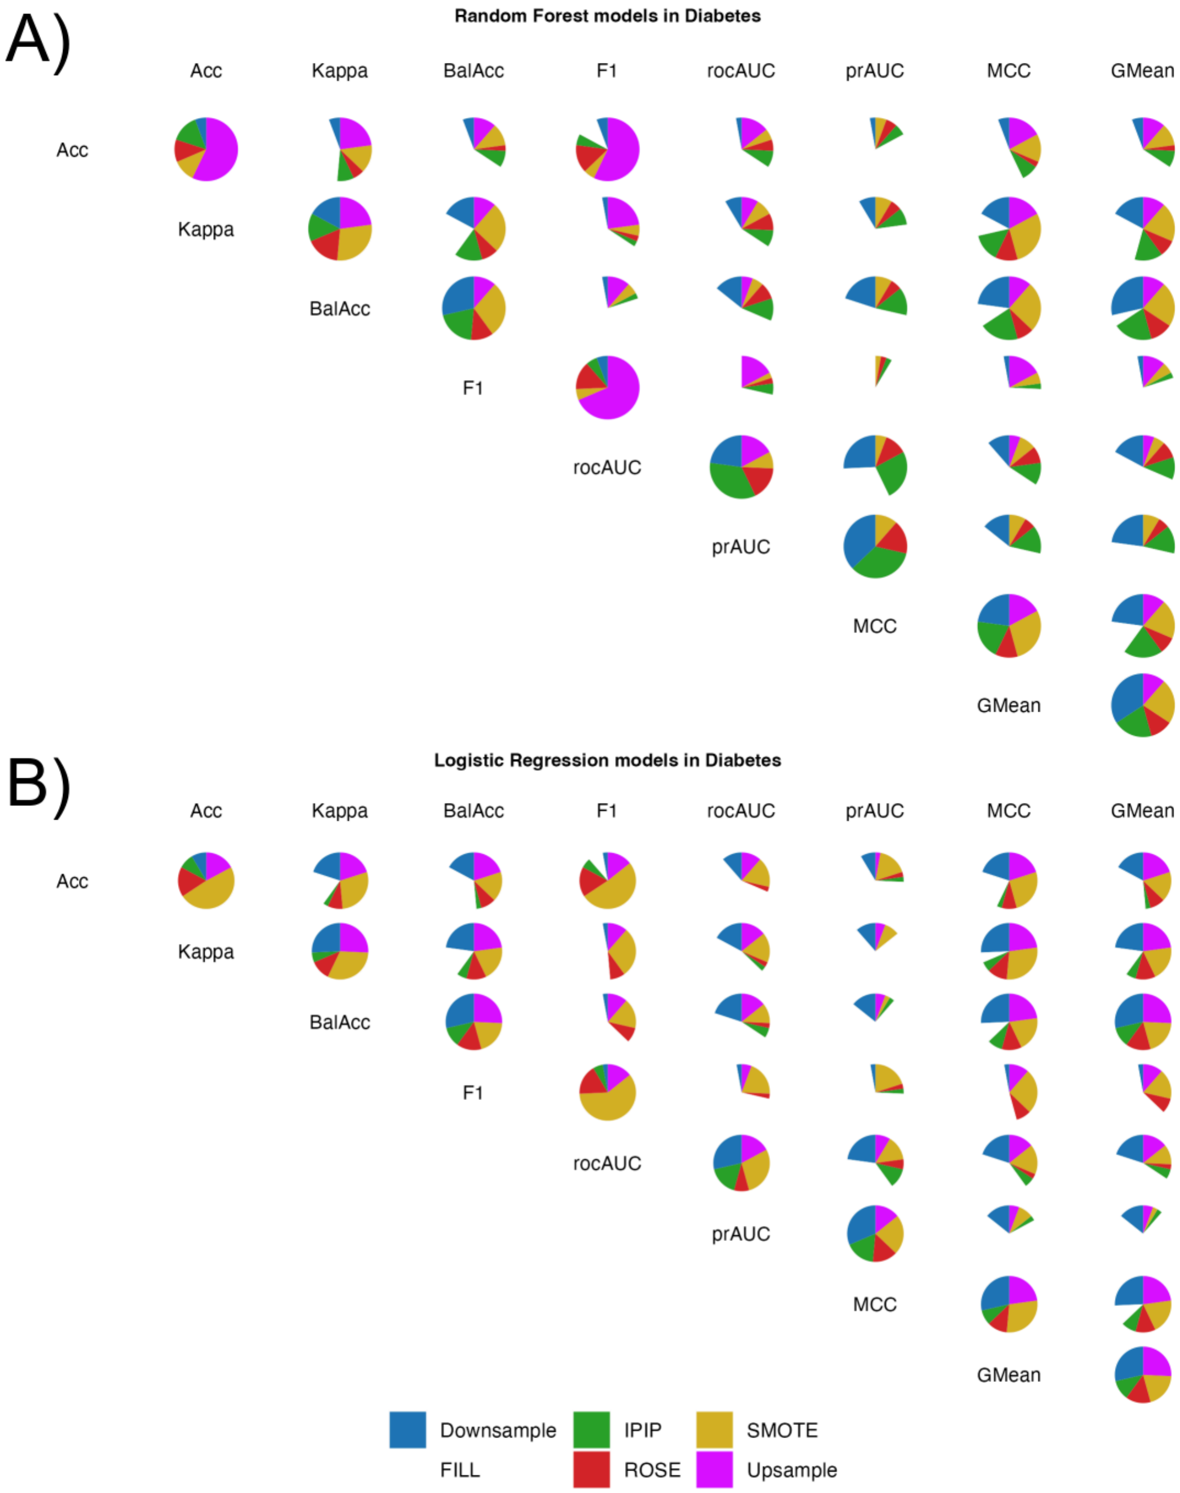


Supplementary Figure S6: A) Concordance plot of the Diabetes dataset using Random Forest. B) Concordance plot of the Diabetes dataset using Logistic Regression models.

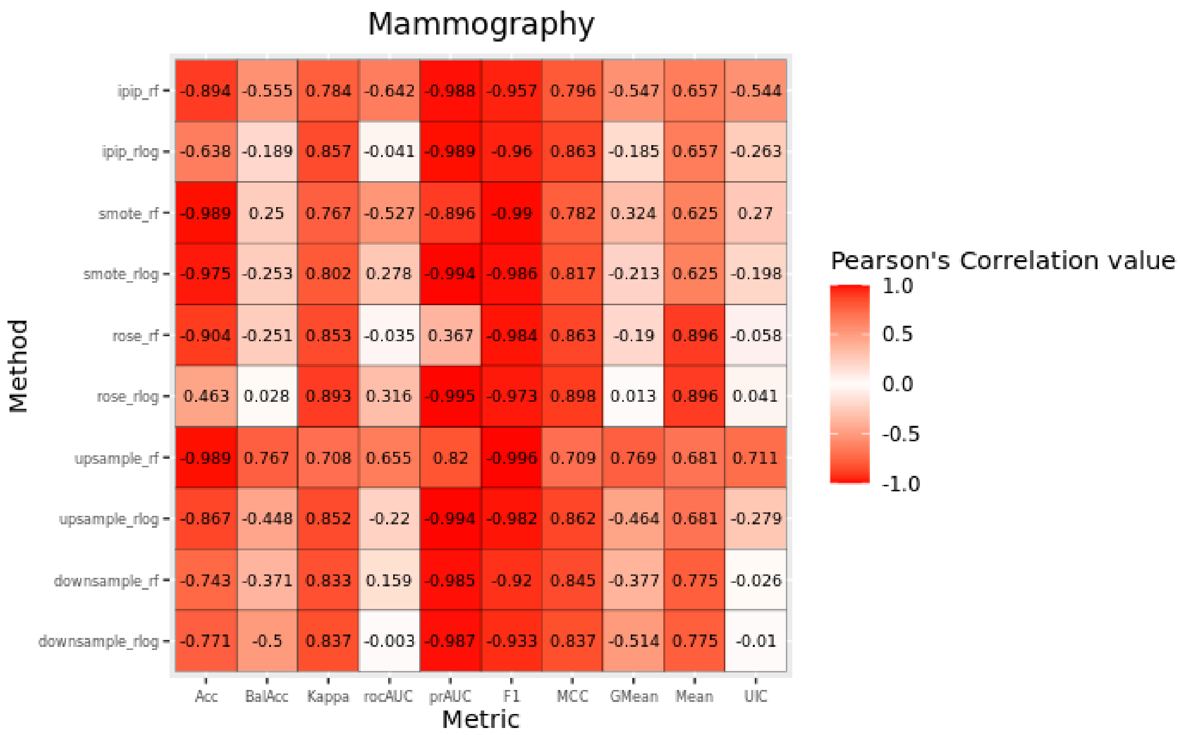


Supplementary Figure S7: Correlation heatmaps beetwen metrics and $p_{min}$ in Mammography dataset.

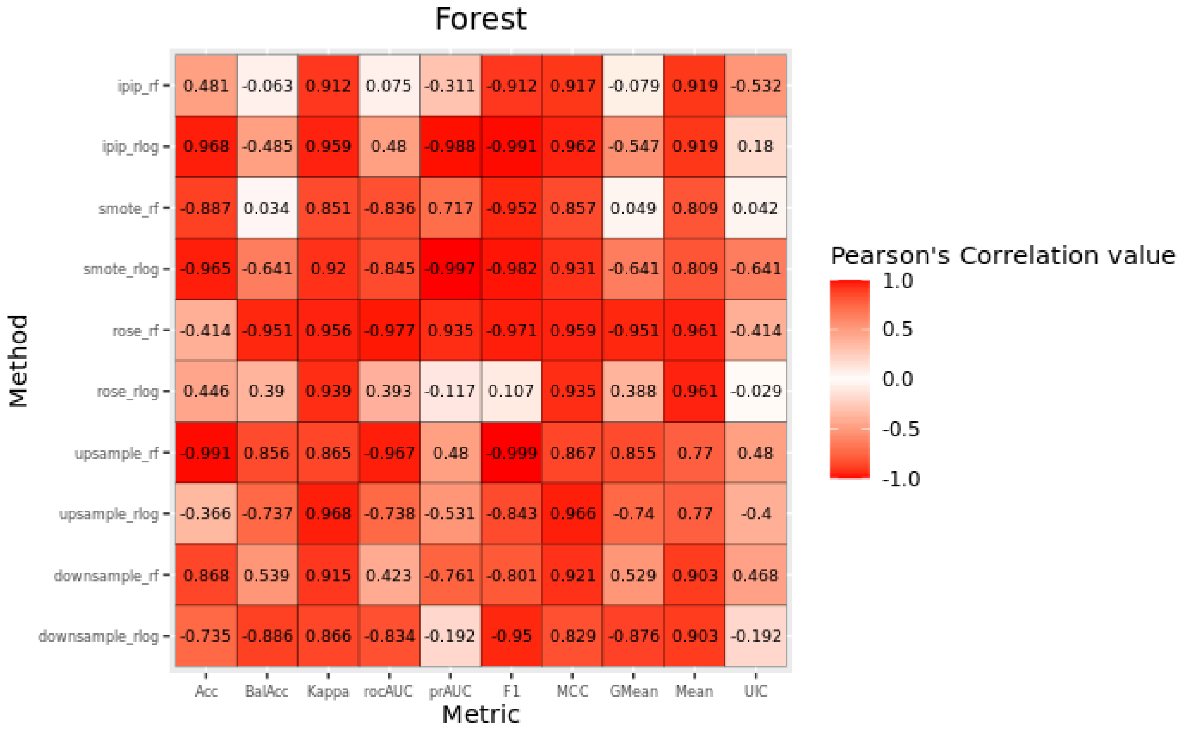


Supplementary Figure S8: Correlation heatmaps beetwen metrics and $p_{min}$ in Forest dataset.

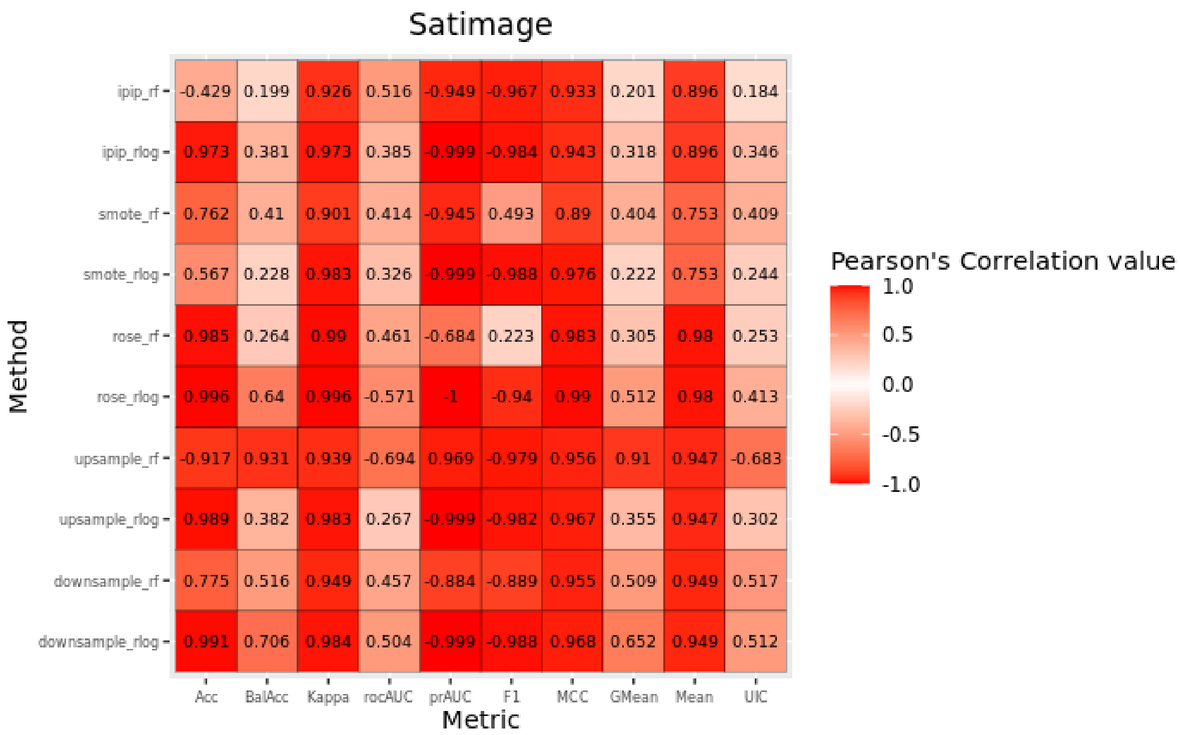


Supplementary Figure S9: Correlation heatmaps beetwen metrics and $p_{min}$ in Satimage dataset.

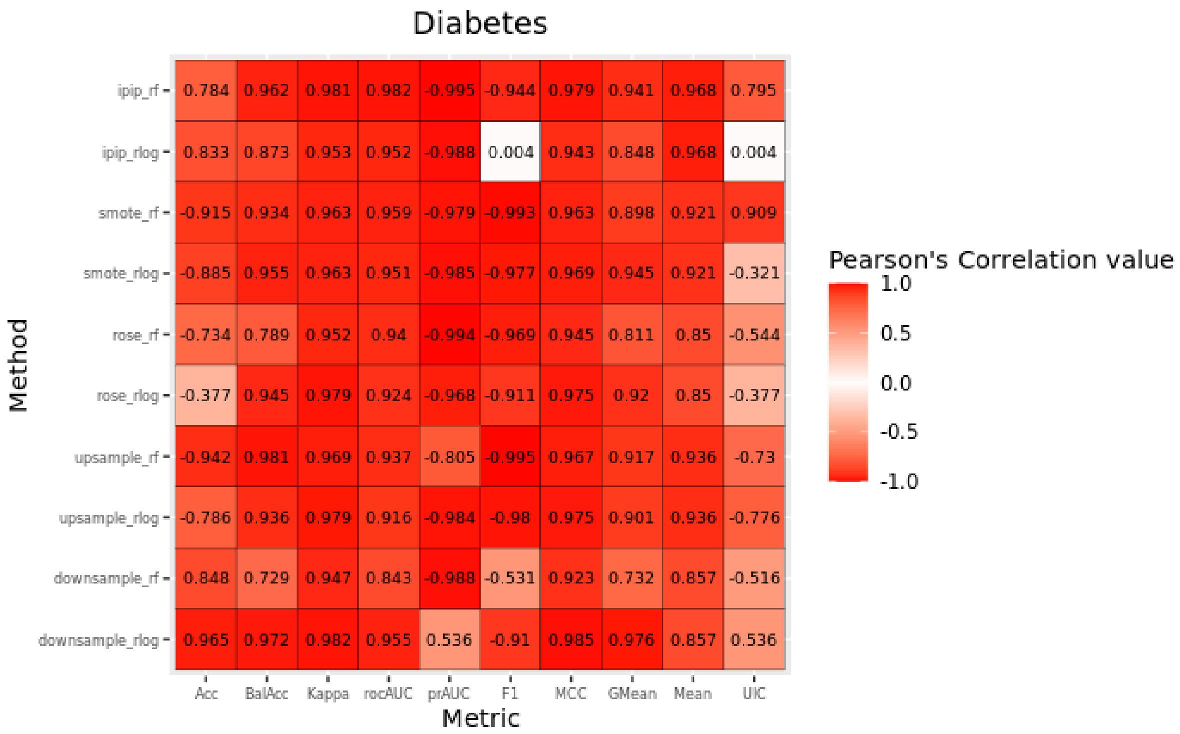


Supplementary Figure S10: Correlation heatmaps beetwen metrics and $p_{min}$ in Diabetes dataset.

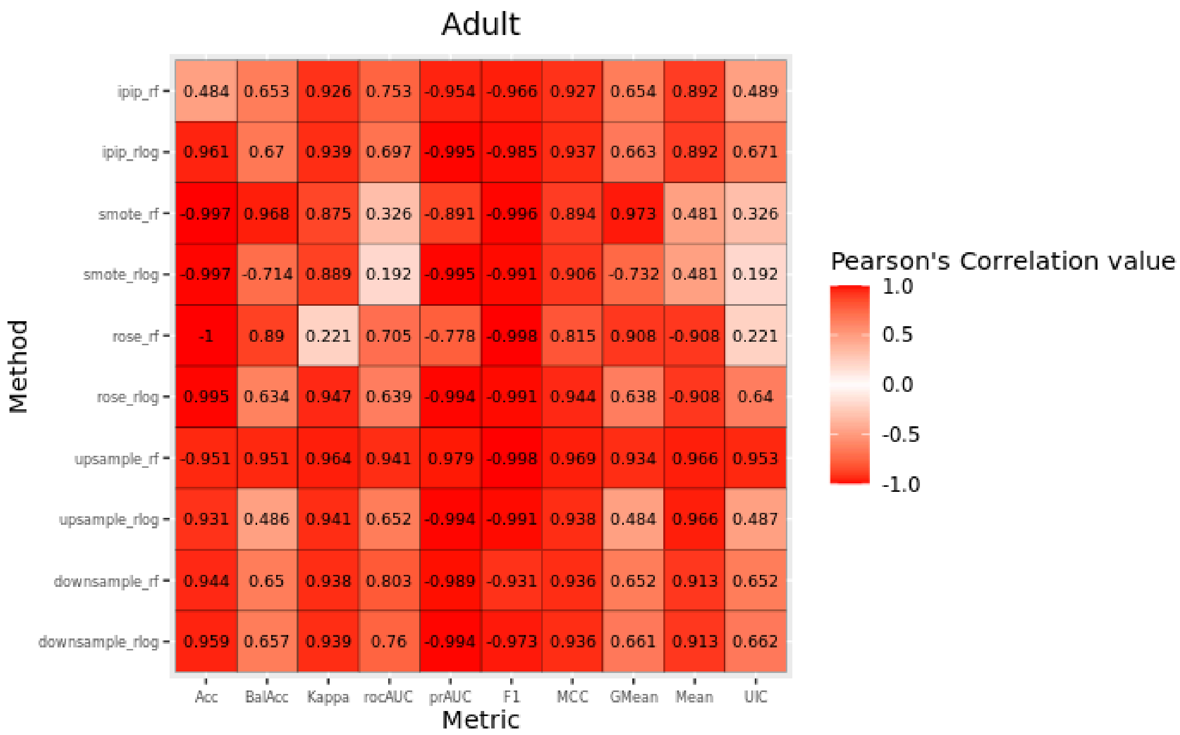


Supplementary Figure S11: Correlation heatmaps beetwen metrics and $p_{min}$ in Adult dataset.

| | mtry | min.node.size | splitrule |
|---|---|---|---|
| **SMS** | {1, 4, 7, 10, 13, 16, 19} | {1, 11, 21} | gini |
| **Mammography** | {1, 2, 3, 4, 5} | {3, 13, 23} | gini |
| **Forest** | {1, 4, 7, 10, 13, 16, 19} | {1, 11, 21} | gini |
| **Satimage** | {1, 3, 5, 7} | {1, 11, 21} | gini |
| **Adult** | {1, 3, 5, 7, 9, 11, 13} | {1, 11, 21} | gini |
| **Phoneme** | {1, 2, 3, 4, 5} | {1, 11, 21} | gini |
| **Diabetes** | {1, 3, 5, 7} | {1, 11, 21} | gini |

Supplementary Table S1: Values given to create the grid of hyperparameters for random forest models in all experiments for each dataset.
